# Supplementary material for: Engagement and Disclosures in LLM-Powered Cognitive Behavioral Therapy Exercises: A Factorial Design Comparing the Influence of a Robot vs. Chatbot Over Time
Source: arXiv:2506.17831 source file (2025-06-21)
Supplement: Supplementary file 1 [file Appendices-standalone.tex]

\documentclass[manuscript,anonymous]{acmart}

\usepackage{array}
\usepackage{multirow}
\usepackage{graphicx}
\usepackage{tabularx}
\usepackage{makecell}
\usepackage{subfig}

\usepackage[utf8]{inputenc}
\usepackage{array}
\usepackage{xcolor}

\begin{document}

\section*{Appendices}

\section{GPT-3.5 Parameters} \label{gpt-parameters}
The input parameters for OpenAI’s chat completion API were:\\
\renewcommand{\thetable}{S1}
\begin{table}[H]
\centering
\begin{tabular}{|l|l|}
\hline
model & gpt-3.5-turbo \\ \hline
messages & <transcript> \\ \hline
stop & Patient \\ \hline
temperature & 1 \\ \hline
frequency\_penalty & 2 \\ \hline
presence\_penalty & 2 \\ \hline
n & 2 \\ \hline
max\_tokens & 150 \\ \hline
\end{tabular}
\caption{\textbf{LLM Parameters.} Model parameters for OpenAI's completion API.}
\label{tab:model_parameters}
\end{table}
The transcript being sent includes all of the previous messages and the user's latest message.

For moderator, the input parameters were same as above, except the temperature was increased to 2 and the values for n and max\_tokens were not sent.

\section{Python Libraries} \label{python-libraries}
\renewcommand{\thetable}{S2}
\begin{table}[H]
\centering
\begin{tabular}{|l|l|}
\hline
pandas & 2.0.2 \\ \hline
matplotlib & 3.7.1 \\ \hline
scipy & 1.10.1 \\ \hline
pingouin & 0.5.3 \\ \hline
numpy & 1.24.3 \\ \hline
\end{tabular}
\caption{\textbf{Python libraries.} The Python libraries used during our analysis and data cleaning.}
\label{tab:python}
\end{table}

\section{R Packages} \label{rpackages}

\begin{table}[H]
\centering
\renewcommand{\thetable}{S3}
\begin{tabular}{|l|l|}
\hline
readxl & 1.4.2 \\ \hline
dplyr & 1.1.2 \\ \hline
tidyr & 1.3.0 \\ \hline
outliers & 0.15 \\ \hline
rstatix & 0.7.2 \\ \hline
ggpubr & 0.6.0 \\ \hline
car & 3.1-2 \\ \hline
lmtest & 0.9-40 \\ \hline
DescTools & 0.99.49 \\ \hline
ggplot2 & 3.4.2 \\ \hline
ggcorrplot & 0.1.4 \\ \hline
MASS & 7.3-60 \\ \hline
afex & 1.3-0 \\ \hline
pastecs & 1.4.2 \\ \hline
ez & 4.4-0 \\ \hline
reshape & 0.8.9 \\ \hline
\end{tabular}
\caption{\textbf{R packages.} The R packages used during our statistical analysis.}
\label{tab:r}
\end{table}

\end{document}
